# Supplementary material for: Self-calibrating Deep Photometric Stereo Networks
Source: arXiv:1903.07366 source file (2019-03-18)
Supplement: Supplementary file 1 [file qual_stage.tex]

\makebox[0.15\textwidth]{\small Objects} 
    \makebox[0.15\textwidth]{\small UPS-FCN \cite{chen2018ps}}
    \makebox[0.15\textwidth]{\small UPS-FCN$_\text{deep+mask}$} 
    \makebox[0.15\textwidth]{\small SDPS-Net} 
    \makebox[0.10\textwidth]{\small SDPS-Net Dir. Err.} 
    \\
    \raisebox{0.2\height}{\rotatebox{90}{\small (a) Helmet Side}}
    \includegraphics[width=0.148\textwidth]{images/Results/LightStage/{4.0_helmet_side_left_0192}.png}
    \includegraphics[width=0.148\textwidth]{images/Results/LightStage/UPS-FCN_ECCV/helmet_side_left_Normal_DiLiGenT}
    \includegraphics[width=0.148\textwidth]{images/Results/LightStage/End_to_end/helmet_side_left_Normal_DiLiGenT}
    \includegraphics[width=0.148\textwidth]{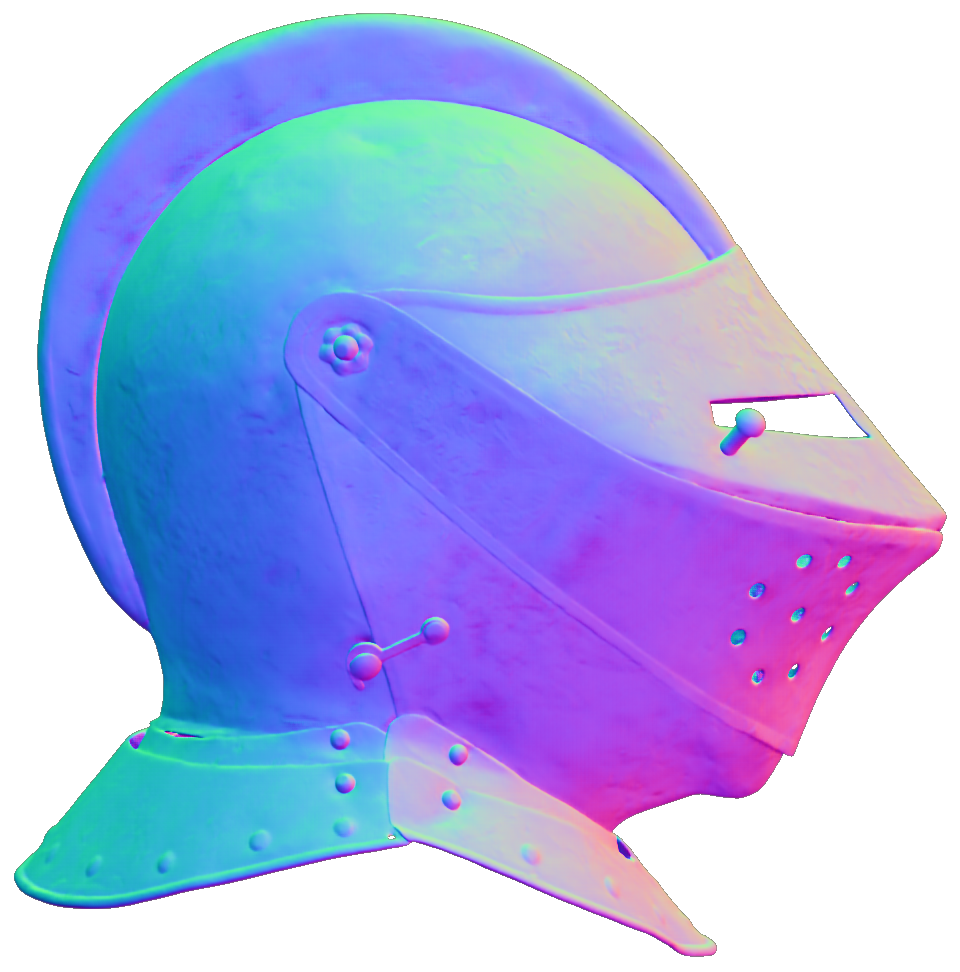}
    \raisebox{0.2\height}{\includegraphics[width=0.10\textwidth]{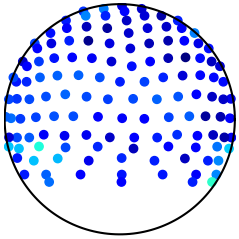}}
    \begin{minipage}{0.012\textwidth} \centering
         \vspace{-6em} \makebox[0.16\textwidth]{\tiny $0\degree$}\\ \vspace{0.2em}
         \includegraphics[width=0.6\linewidth]{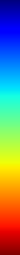} \\ \vspace{-0.4em}
         \makebox[0.16\textwidth]{\tiny$45\degree$}\\
    \end{minipage}
    \\
    \raisebox{0.5\height}{\rotatebox{90}{\small (b) Helmet Front}}
    \includegraphics[width=0.148\textwidth]{images/Results/LightStage/{4.0_helmet_front_left_0082}.png}
    \includegraphics[width=0.148\textwidth]{images/Results/LightStage/UPS-FCN_ECCV/helmet_front_left_Normal_DiLiGenT}
    \includegraphics[width=0.148\textwidth]{images/Results/LightStage/End_to_end/helmet_front_left_Normal_DiLiGenT}
    \includegraphics[width=0.148\textwidth]{images/Results/LightStage/SCPS/helmet_front_left_Normal_DiLiGenT}
    \raisebox{0.6\height}{\includegraphics[width=0.10\textwidth]{images/Results/LightStage/SCPS/helmet_front_left}}
    \begin{minipage}{0.012\textwidth} \centering
         \vspace{-10em} \makebox[0.16\textwidth]{\tiny $0\degree$}\\ \vspace{0.2em}
         \includegraphics[width=0.6\linewidth]{images/Results/color_bar} \\ \vspace{-0.4em}
         \makebox[0.16\textwidth]{\tiny$45\degree$}\\
    \end{minipage}
    \\
    \raisebox{0.5\height}{\rotatebox{90}{\small (c) Fighting Knight}}
    \includegraphics[width=0.148\textwidth]{images/Results/LightStage/{4.0_knight_fighting_057}.png}
    \includegraphics[width=0.148\textwidth]{images/Results/LightStage/UPS-FCN_ECCV/knight_fighting_Normal_DiLiGenT}
    \includegraphics[width=0.148\textwidth]{images/Results/LightStage/End_to_end/knight_fighting_Normal_DiLiGenT}
    \includegraphics[width=0.148\textwidth]{images/Results/LightStage/SCPS/knight_fighting_Normal_DiLiGenT}
    \raisebox{0.8\height}{\includegraphics[width=0.10\textwidth]{images/Results/LightStage/SCPS/knight_fighting}}
    \begin{minipage}{0.012\textwidth} \centering
         \vspace{-12em} \makebox[0.16\textwidth]{\tiny $0\degree$}\\ \vspace{0.2em}
         \includegraphics[width=0.6\linewidth]{images/Results/color_bar} \\ \vspace{-0.4em}
         \makebox[0.16\textwidth]{\tiny$45\degree$}\\
    \end{minipage}
    \\
    \raisebox{0.0\height}{\rotatebox{90}{\footnotesize (d) Kneeling Knight}}
    \includegraphics[width=0.148\textwidth]{images/Results/LightStage/{4.0_knight_kneeling_048}.png}
    \includegraphics[width=0.148\textwidth]{images/Results/LightStage/UPS-FCN_ECCV/knight_kneeling_Normal_DiLiGenT}
    \includegraphics[width=0.148\textwidth]{images/Results/LightStage/End_to_end/knight_kneeling_Normal_DiLiGenT}
    \includegraphics[width=0.148\textwidth]{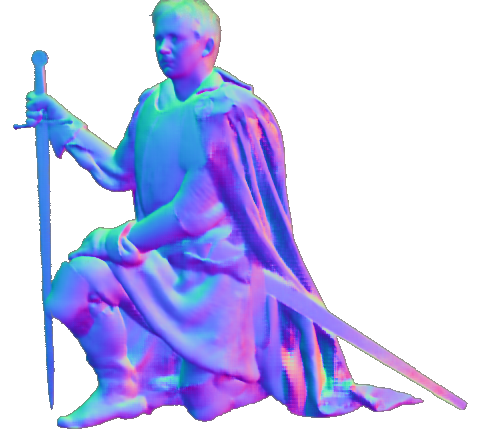}
    \raisebox{0.2\height}{\includegraphics[width=0.10\textwidth]{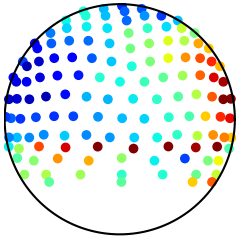}}
    \begin{minipage}{0.012\textwidth} \centering
         \vspace{-6em} \makebox[0.16\textwidth]{\tiny $0\degree$}\\ \vspace{0.2em}
         \includegraphics[width=0.6\linewidth]{images/Results/color_bar} \\ \vspace{-0.4em}
         \makebox[0.16\textwidth]{\tiny$45\degree$}\\
    \end{minipage}
    \\
    \raisebox{0.2\height}{\rotatebox{90}{\small (e) Standing Knight}}
    \includegraphics[width=0.148\textwidth]{images/Results/LightStage/{4.0_knight_standing_116}.png}
    \includegraphics[width=0.148\textwidth]{images/Results/LightStage/UPS-FCN_ECCV/knight_standing_Normal_DiLiGenT}
    \includegraphics[width=0.148\textwidth]{images/Results/LightStage/End_to_end/knight_standing_Normal_DiLiGenT}
    \includegraphics[width=0.148\textwidth]{images/Results/LightStage/SCPS/knight_standing_Normal_DiLiGenT}
    \raisebox{0.6\height}{\includegraphics[width=0.10\textwidth]{images/Results/LightStage/SCPS/knight_standing}}
    \begin{minipage}{0.012\textwidth} \centering
         \vspace{-10em} \makebox[0.16\textwidth]{\tiny $0\degree$}\\ \vspace{0.2em}
         \includegraphics[width=0.6\linewidth]{images/Results/color_bar} \\ \vspace{-0.4em}
         \makebox[0.16\textwidth]{\tiny$45\degree$}\\
    \end{minipage}
    \\
    \raisebox{0.4\height}{\rotatebox{90}{\small (d) Plant}}
    \includegraphics[width=0.148\textwidth]{images/Results/LightStage/{2.0_plant_left_0021}}
    \includegraphics[width=0.148\textwidth]{images/Results/LightStage/UPS-FCN_ECCV/plant_left_Normal_DiLiGenT}
    \includegraphics[width=0.148\textwidth]{images/Results/LightStage/End_to_end/plant_left_Normal_DiLiGenT}
    \includegraphics[width=0.148\textwidth]{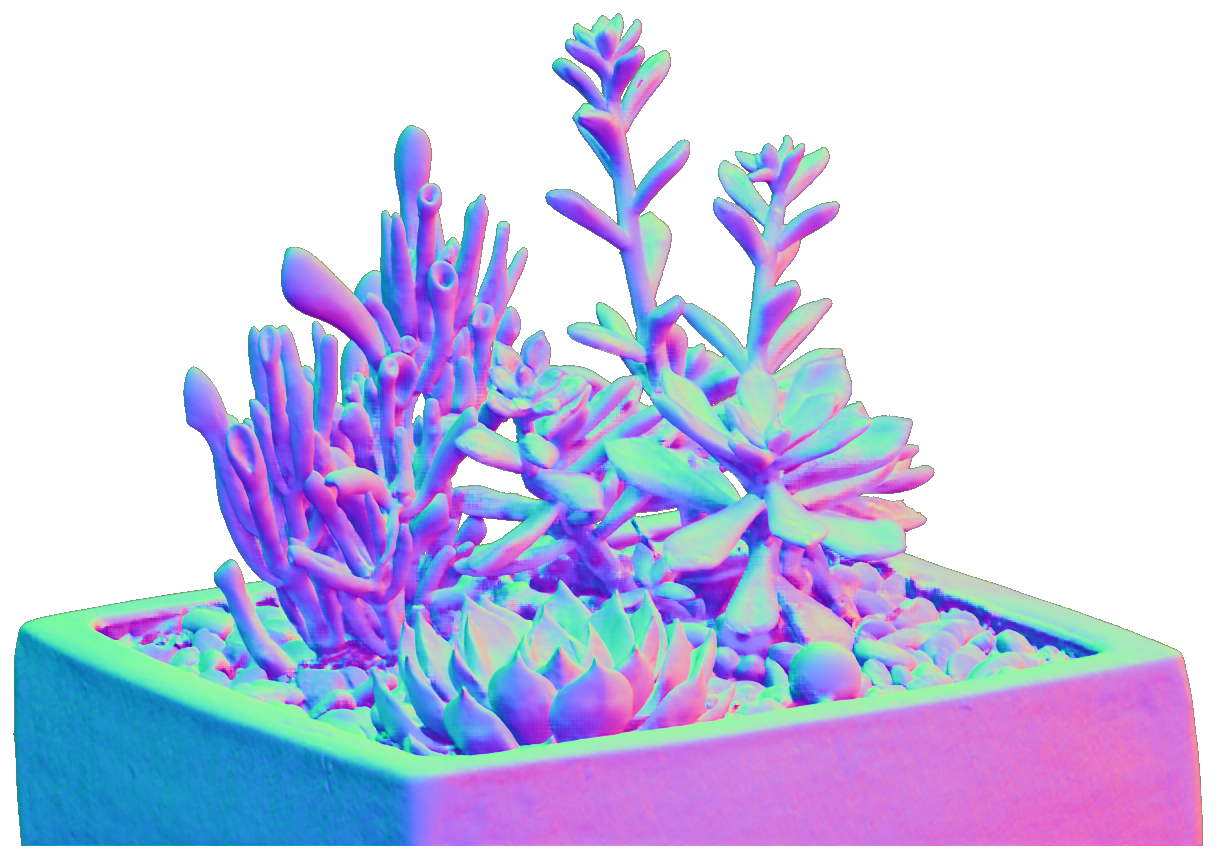}
    \raisebox{0.0\height}{\includegraphics[width=0.10\textwidth]{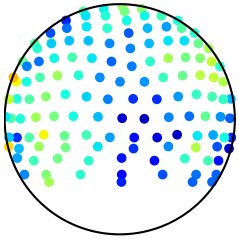}}
    \begin{minipage}{0.012\textwidth} \centering
         \vspace{-6em} \makebox[0.16\textwidth]{\tiny $0\degree$}\\ \vspace{0.2em}
         \includegraphics[width=0.6\linewidth]{images/Results/color_bar} \\ \vspace{-0.4em}
         \makebox[0.16\textwidth]{\tiny$45\degree$}\\
    \end{minipage}
    \\
