# Supplementary material for: Self-calibrating Deep Photometric Stereo Networks
Source: arXiv:1903.07366 source file (2019-03-18)
Supplement: Supplementary file 2 [file res_qual_diligent_compare.tex]

\begin{minipage}{0.97\textwidth}\centering
 \makebox[0.15\textwidth]{\small GT / Object} 
 \makebox[0.15\textwidth]{\small SDPS-Net} 
 \makebox[0.15\textwidth]{\small UPS-FCN$_\text{deep+mask}$} 
 \makebox[0.15\textwidth]{\small UPS-FCN \cite{chen2018ps}}
 \makebox[0.15\textwidth]{\small PF14 \cite{papad14closed}} 
 \makebox[0.15\textwidth]{\small WT13 \cite{wu2013calib}} 
  \\
 \includegraphics[width=0.15\textwidth]{images/Results/DiLiGenT/GT/ballPNGGT_normal}
 \includegraphics[width=0.15\textwidth]{images/Results/DiLiGenT/SCPS/ballPNGDiLiGenT_normal}
 \includegraphics[width=0.15\textwidth]{images/Results/DiLiGenT/End_to_end/ballPNGDiLiGenT_normal}
 \includegraphics[width=0.15\textwidth]{images/Results/DiLiGenT/UPS-FCN_ECCV/ballPNGDiLiGenT_normal}
 \includegraphics[width=0.15\textwidth]{images/Results/DiLiGenT/compare/ballPNGCVPR12Favaro_normal}
 \includegraphics[width=0.15\textwidth]{images/Results/DiLiGenT/compare/ballPNGCVPR13Wu_normal}
  \\
  \includegraphics[width=0.15\textwidth]{images/Results/DiLiGenT/GT/{4.0_ballPNG_001}.png}
 \includegraphics[width=0.15\textwidth]{images/Results/DiLiGenT/SCPS/ballPNGDiLiGenT_diff}
 \includegraphics[width=0.15\textwidth]{images/Results/DiLiGenT/End_to_end/ballPNGDiLiGenT_diff}
 \includegraphics[width=0.15\textwidth]{images/Results/DiLiGenT/UPS-FCN_ECCV/ballPNGDiLiGenT_diff}
 \includegraphics[width=0.15\textwidth]{images/Results/DiLiGenT/compare/ballPNGCVPR12Favaro_diff}
 \includegraphics[width=0.15\textwidth]{images/Results/DiLiGenT/compare/ballPNGCVPR13Wu_diff}\\
 \makebox[0.15\textwidth]{\small (a) {\sc ball}} 
 \makebox[0.15\textwidth]{\small 2.77} 
 \makebox[0.15\textwidth]{\small 3.96} 
 \makebox[0.15\textwidth]{\small 6.62} 
 \makebox[0.15\textwidth]{\small 4.77} 
 \makebox[0.15\textwidth]{\small 4.39} 
  \\
  \vspace{1em}
 \includegraphics[width=0.15\textwidth]{images/Results/DiLiGenT/GT/catPNGGT_normal}
 \includegraphics[width=0.15\textwidth]{images/Results/DiLiGenT/SCPS/catPNGDiLiGenT_normal}
 \includegraphics[width=0.15\textwidth]{images/Results/DiLiGenT/End_to_end/catPNGDiLiGenT_normal}
 \includegraphics[width=0.15\textwidth]{images/Results/DiLiGenT/UPS-FCN_ECCV/catPNGDiLiGenT_normal}
 \includegraphics[width=0.15\textwidth]{images/Results/DiLiGenT/compare/catPNGCVPR12Favaro_normal}
 \includegraphics[width=0.15\textwidth]{images/Results/DiLiGenT/compare/catPNGCVPR13Wu_normal}
  \\
  \includegraphics[width=0.15\textwidth]{images/Results/DiLiGenT/GT/{4.0_catPNG_001}.png}
 \includegraphics[width=0.15\textwidth]{images/Results/DiLiGenT/SCPS/catPNGDiLiGenT_diff}
 \includegraphics[width=0.15\textwidth]{images/Results/DiLiGenT/End_to_end/catPNGDiLiGenT_diff}
 \includegraphics[width=0.15\textwidth]{images/Results/DiLiGenT/UPS-FCN_ECCV/catPNGDiLiGenT_diff}
 \includegraphics[width=0.15\textwidth]{images/Results/DiLiGenT/compare/catPNGCVPR12Favaro_diff}
 \includegraphics[width=0.15\textwidth]{images/Results/DiLiGenT/compare/catPNGCVPR13Wu_diff}\\
 \makebox[0.15\textwidth]{\small (b) {\sc cat}} 
 \makebox[0.15\textwidth]{\small 8.06} 
 \makebox[0.15\textwidth]{\small 12.16} 
 \makebox[0.15\textwidth]{\small 14.68} 
 \makebox[0.15\textwidth]{\small 9.54} 
 \makebox[0.15\textwidth]{\small 36.55} 
  \\
  \vspace{1em}
 \includegraphics[width=0.15\textwidth]{images/Results/DiLiGenT/GT/bearPNGGT_normal}
 \includegraphics[width=0.15\textwidth]{images/Results/DiLiGenT/SCPS/bearPNGDiLiGenT_normal}
 \includegraphics[width=0.15\textwidth]{images/Results/DiLiGenT/End_to_end/bearPNGDiLiGenT_normal}
 \includegraphics[width=0.15\textwidth]{images/Results/DiLiGenT/UPS-FCN_ECCV/bearPNGDiLiGenT_normal}
 \includegraphics[width=0.15\textwidth]{images/Results/DiLiGenT/compare/bearPNGCVPR12Favaro_normal}
 \includegraphics[width=0.15\textwidth]{images/Results/DiLiGenT/compare/bearPNGCVPR13Wu_normal}
  \\
  \includegraphics[width=0.15\textwidth]{images/Results/DiLiGenT/GT/{4.0_bearPNG_001}.png}
 \includegraphics[width=0.15\textwidth]{images/Results/DiLiGenT/SCPS/bearPNGDiLiGenT_diff}
 \includegraphics[width=0.15\textwidth]{images/Results/DiLiGenT/End_to_end/bearPNGDiLiGenT_diff}
 \includegraphics[width=0.15\textwidth]{images/Results/DiLiGenT/UPS-FCN_ECCV/bearPNGDiLiGenT_diff}
 \includegraphics[width=0.15\textwidth]{images/Results/DiLiGenT/compare/bearPNGCVPR12Favaro_diff}
 \includegraphics[width=0.15\textwidth]{images/Results/DiLiGenT/compare/bearPNGCVPR13Wu_diff}\\
 \makebox[0.15\textwidth]{\small (c) {\sc bear}} 
 \makebox[0.15\textwidth]{\small 6.89} 
 \makebox[0.15\textwidth]{\small 7.19} 
 \makebox[0.15\textwidth]{\small 11.23} 
 \makebox[0.15\textwidth]{\small 9.07} 
 \makebox[0.15\textwidth]{\small 6.42} 
\end{minipage}
    \begin{minipage}{0.02\textwidth} \centering
         \makebox[0.16\textwidth]{\small $0\degree$}\\ \vspace{0.2em}
         \includegraphics[width=\linewidth]{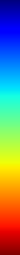} \\ \vspace{-0.4em}
         \makebox[0.16\textwidth]{\small$90\degree$}\\
    \end{minipage}
    \\
