# Supplementary material for: Self-calibrating Deep Photometric Stereo Networks
Source: arXiv:1903.07366 source file (2019-03-18)
Supplement: Supplementary file 3 [file res_qual_diligent_compare2.tex]

\begin{minipage}{0.97\textwidth}\centering
 \makebox[0.15\textwidth]{\small GT / Object} 
 \makebox[0.15\textwidth]{\small SDPS-Net} 
 \makebox[0.15\textwidth]{\small UPS-FCN$_\text{deep+mask}$} 
 \makebox[0.15\textwidth]{\small UPS-FCN \cite{chen2018ps}}
 \makebox[0.15\textwidth]{\small PF14 \cite{papad14closed}} 
 \makebox[0.15\textwidth]{\small WT13 \cite{wu2013calib}} 
  \\
 \includegraphics[width=0.15\textwidth]{images/Results/DiLiGenT/GT/pot2PNGGT_normal}
 \includegraphics[width=0.15\textwidth]{images/Results/DiLiGenT/SCPS/pot2PNGDiLiGenT_normal}
 \includegraphics[width=0.15\textwidth]{images/Results/DiLiGenT/End_to_end/pot2PNGDiLiGenT_normal}
 \includegraphics[width=0.15\textwidth]{images/Results/DiLiGenT/UPS-FCN_ECCV/pot2PNGDiLiGenT_normal}
 \includegraphics[width=0.15\textwidth]{images/Results/DiLiGenT/compare/pot2PNGCVPR12Favaro_normal}
 \includegraphics[width=0.15\textwidth]{images/Results/DiLiGenT/compare/pot2PNGCVPR13Wu_normal}
  \\
  \includegraphics[width=0.15\textwidth]{images/Results/DiLiGenT/GT/{4.0_pot2PNG_001}.png}
 \includegraphics[width=0.15\textwidth]{images/Results/DiLiGenT/SCPS/pot2PNGDiLiGenT_diff}
 \includegraphics[width=0.15\textwidth]{images/Results/DiLiGenT/End_to_end/pot2PNGDiLiGenT_diff}
 \includegraphics[width=0.15\textwidth]{images/Results/DiLiGenT/UPS-FCN_ECCV/pot2PNGDiLiGenT_diff}
 \includegraphics[width=0.15\textwidth]{images/Results/DiLiGenT/compare/pot2PNGCVPR12Favaro_diff}
 \includegraphics[width=0.15\textwidth]{images/Results/DiLiGenT/compare/pot2PNGCVPR13Wu_diff}\\
 \makebox[0.15\textwidth]{\small (a) {\sc pot2}} 
 \makebox[0.15\textwidth]{\small 7.50} 
 \makebox[0.15\textwidth]{\small 11.11} 
 \makebox[0.15\textwidth]{\small 14.19} 
 \makebox[0.15\textwidth]{\small 15.90} 
 \makebox[0.15\textwidth]{\small 14.52} 
  \\
  \vspace{1em}
 \includegraphics[width=0.15\textwidth]{images/Results/DiLiGenT/GT/buddhaPNGGT_normal}
 \includegraphics[width=0.15\textwidth]{images/Results/DiLiGenT/SCPS/buddhaPNGDiLiGenT_normal}
 \includegraphics[width=0.15\textwidth]{images/Results/DiLiGenT/End_to_end/buddhaPNGDiLiGenT_normal}
 \includegraphics[width=0.15\textwidth]{images/Results/DiLiGenT/UPS-FCN_ECCV/buddhaPNGDiLiGenT_normal}
 \includegraphics[width=0.15\textwidth]{images/Results/DiLiGenT/compare/buddhaPNGCVPR12Favaro_normal}
 \includegraphics[width=0.15\textwidth]{images/Results/DiLiGenT/compare/buddhaPNGCVPR13Wu_normal}
  \\
  \includegraphics[width=0.15\textwidth]{images/Results/DiLiGenT/GT/{4.0_buddhaPNG_001}.png}
 \includegraphics[width=0.15\textwidth]{images/Results/DiLiGenT/SCPS/buddhaPNGDiLiGenT_diff}
 \includegraphics[width=0.15\textwidth]{images/Results/DiLiGenT/End_to_end/buddhaPNGDiLiGenT_diff}
 \includegraphics[width=0.15\textwidth]{images/Results/DiLiGenT/UPS-FCN_ECCV/buddhaPNGDiLiGenT_diff}
 \includegraphics[width=0.15\textwidth]{images/Results/DiLiGenT/compare/buddhaPNGCVPR12Favaro_diff}
 \includegraphics[width=0.15\textwidth]{images/Results/DiLiGenT/compare/buddhaPNGCVPR13Wu_diff}\\
 \makebox[0.15\textwidth]{\small (b) {\sc buddha}} 
 \makebox[0.15\textwidth]{\small 8.97} 
 \makebox[0.15\textwidth]{\small 13.06}
 \makebox[0.15\textwidth]{\small 15.87}
 \makebox[0.15\textwidth]{\small 14.92}
 \makebox[0.15\textwidth]{\small 13.19}
  \\
  \vspace{1em}
 \includegraphics[width=0.15\textwidth]{images/Results/DiLiGenT/GT/gobletPNGGT_normal}
 \includegraphics[width=0.15\textwidth]{images/Results/DiLiGenT/SCPS/gobletPNGDiLiGenT_normal}
 \includegraphics[width=0.15\textwidth]{images/Results/DiLiGenT/End_to_end/gobletPNGDiLiGenT_normal}
 \includegraphics[width=0.15\textwidth]{images/Results/DiLiGenT/UPS-FCN_ECCV/gobletPNGDiLiGenT_normal}
 \includegraphics[width=0.15\textwidth]{images/Results/DiLiGenT/compare/gobletPNGCVPR12Favaro_normal}
 \includegraphics[width=0.15\textwidth]{images/Results/DiLiGenT/compare/gobletPNGCVPR13Wu_normal}
  \\
  \includegraphics[width=0.15\textwidth]{images/Results/DiLiGenT/GT/{4.0_gobletPNG_001}.png}
 \includegraphics[width=0.15\textwidth]{images/Results/DiLiGenT/SCPS/gobletPNGDiLiGenT_diff}
 \includegraphics[width=0.15\textwidth]{images/Results/DiLiGenT/End_to_end/gobletPNGDiLiGenT_diff}
 \includegraphics[width=0.15\textwidth]{images/Results/DiLiGenT/UPS-FCN_ECCV/gobletPNGDiLiGenT_diff}
 \includegraphics[width=0.15\textwidth]{images/Results/DiLiGenT/compare/gobletPNGCVPR12Favaro_diff}
 \includegraphics[width=0.15\textwidth]{images/Results/DiLiGenT/compare/gobletPNGCVPR13Wu_diff}\\
 \makebox[0.15\textwidth]{\small (c) {\sc goblet}} 
 \makebox[0.15\textwidth]{\small 11.91} 
 \makebox[0.15\textwidth]{\small 18.07}
 \makebox[0.15\textwidth]{\small 20.72}
 \makebox[0.15\textwidth]{\small 29.93}
 \makebox[0.15\textwidth]{\small 20.57}
\end{minipage}
    \begin{minipage}{0.02\textwidth} \centering
         \makebox[0.16\textwidth]{\small $0\degree$}\\ \vspace{0.2em}
         \includegraphics[width=\linewidth]{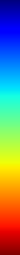} \\ \vspace{-0.4em}
         \makebox[0.16\textwidth]{\small$90\degree$}\\
    \end{minipage}
    \\
