# Supplementary material for: Self-calibrating Deep Photometric Stereo Networks
Source: arXiv:1903.07366 source file (2019-03-18)
Supplement: Supplementary file 4 [file res_qual_diligent_compare3.tex]

\begin{minipage}{0.97\textwidth}\centering
 \makebox[0.15\textwidth]{\small GT / Object} 
 \makebox[0.15\textwidth]{\small SDPS-Net} 
 \makebox[0.15\textwidth]{\small UPS-FCN$_\text{deep+mask}$} 
 \makebox[0.15\textwidth]{\small UPS-FCN \cite{chen2018ps}}
 \makebox[0.15\textwidth]{\small PF14 \cite{papad14closed}} 
 \makebox[0.15\textwidth]{\small WT13 \cite{wu2013calib}} 
  \\
  \vspace{1em}
 \includegraphics[width=0.15\textwidth]{images/Results/DiLiGenT/GT/pot1PNGGT_normal}
 \includegraphics[width=0.15\textwidth]{images/Results/DiLiGenT/SCPS/pot1PNGDiLiGenT_normal}
 \includegraphics[width=0.15\textwidth]{images/Results/DiLiGenT/End_to_end/pot1PNGDiLiGenT_normal}
 \includegraphics[width=0.15\textwidth]{images/Results/DiLiGenT/UPS-FCN_ECCV/pot1PNGDiLiGenT_normal}
 \includegraphics[width=0.15\textwidth]{images/Results/DiLiGenT/compare/pot1PNGCVPR12Favaro_normal}
 \includegraphics[width=0.15\textwidth]{images/Results/DiLiGenT/compare/pot1PNGCVPR13Wu_normal}
  \\
  \includegraphics[width=0.15\textwidth]{images/Results/DiLiGenT/GT/{4.0_pot1PNG_001}.png}
 \includegraphics[width=0.15\textwidth]{images/Results/DiLiGenT/SCPS/pot1PNGDiLiGenT_diff}
 \includegraphics[width=0.15\textwidth]{images/Results/DiLiGenT/End_to_end/pot1PNGDiLiGenT_diff}
 \includegraphics[width=0.15\textwidth]{images/Results/DiLiGenT/UPS-FCN_ECCV/pot1PNGDiLiGenT_diff}
 \includegraphics[width=0.15\textwidth]{images/Results/DiLiGenT/compare/pot1PNGCVPR12Favaro_diff}
 \includegraphics[width=0.15\textwidth]{images/Results/DiLiGenT/compare/pot1PNGCVPR13Wu_diff}\\
 \makebox[0.15\textwidth]{\small (a) {\sc pot1}} 
 \makebox[0.15\textwidth]{\small 8.14} 
 \makebox[0.15\textwidth]{\small 11.13} 
 \makebox[0.15\textwidth]{\small 13.98} 
 \makebox[0.15\textwidth]{\small 9.51} 
 \makebox[0.15\textwidth]{\small 9.39} 
  \\
  \vspace{1em}
 \includegraphics[width=0.15\textwidth]{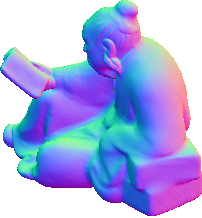}
 \includegraphics[width=0.15\textwidth]{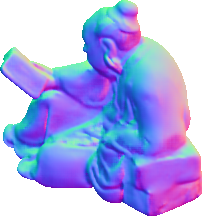}
 \includegraphics[width=0.15\textwidth]{images/Results/DiLiGenT/End_to_end/readingPNGDiLiGenT_normal}
 \includegraphics[width=0.15\textwidth]{images/Results/DiLiGenT/UPS-FCN_ECCV/readingPNGDiLiGenT_normal}
 \includegraphics[width=0.15\textwidth]{images/Results/DiLiGenT/compare/readingPNGCVPR12Favaro_normal}
 \includegraphics[width=0.15\textwidth]{images/Results/DiLiGenT/compare/readingPNGCVPR13Wu_normal}
  \\
  \includegraphics[width=0.15\textwidth]{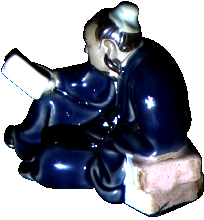}
 \includegraphics[width=0.15\textwidth]{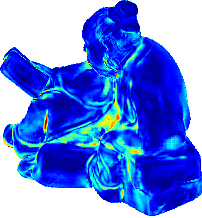}
 \includegraphics[width=0.15\textwidth]{images/Results/DiLiGenT/End_to_end/readingPNGDiLiGenT_diff}
 \includegraphics[width=0.15\textwidth]{images/Results/DiLiGenT/UPS-FCN_ECCV/readingPNGDiLiGenT_diff}
 \includegraphics[width=0.15\textwidth]{images/Results/DiLiGenT/compare/readingPNGCVPR12Favaro_diff}
 \includegraphics[width=0.15\textwidth]{images/Results/DiLiGenT/compare/readingPNGCVPR13Wu_diff}\\
 \makebox[0.15\textwidth]{\small (b) {\sc reading}} 
 \makebox[0.15\textwidth]{\small 14.90}
 \makebox[0.15\textwidth]{\small 20.46}
 \makebox[0.15\textwidth]{\small 23.26}
 \makebox[0.15\textwidth]{\small 24.18}
 \makebox[0.15\textwidth]{\small 58.96}
  \\
  \vspace{1em}
 \includegraphics[width=0.15\textwidth]{images/Results/DiLiGenT/GT/cowPNGGT_normal}
 \includegraphics[width=0.15\textwidth]{images/Results/DiLiGenT/SCPS/cowPNGDiLiGenT_normal}
 \includegraphics[width=0.15\textwidth]{images/Results/DiLiGenT/End_to_end/cowPNGDiLiGenT_normal}
 \includegraphics[width=0.15\textwidth]{images/Results/DiLiGenT/UPS-FCN_ECCV/cowPNGDiLiGenT_normal}
 \includegraphics[width=0.15\textwidth]{images/Results/DiLiGenT/compare/cowPNGCVPR12Favaro_normal}
 \includegraphics[width=0.15\textwidth]{images/Results/DiLiGenT/compare/cowPNGCVPR13Wu_normal}
  \\
  \includegraphics[width=0.15\textwidth]{images/Results/DiLiGenT/GT/{4.0_cowPNG_001}.png}
 \includegraphics[width=0.15\textwidth]{images/Results/DiLiGenT/SCPS/cowPNGDiLiGenT_diff}
 \includegraphics[width=0.15\textwidth]{images/Results/DiLiGenT/End_to_end/cowPNGDiLiGenT_diff}
 \includegraphics[width=0.15\textwidth]{images/Results/DiLiGenT/UPS-FCN_ECCV/cowPNGDiLiGenT_diff}
 \includegraphics[width=0.15\textwidth]{images/Results/DiLiGenT/compare/cowPNGCVPR12Favaro_diff}
 \includegraphics[width=0.15\textwidth]{images/Results/DiLiGenT/compare/cowPNGCVPR13Wu_diff}\\
 \makebox[0.15\textwidth]{\small (c) {\sc cow}} 
 \makebox[0.15\textwidth]{\small 8.48} 
 \makebox[0.15\textwidth]{\small 11.84} 
 \makebox[0.15\textwidth]{\small 11.91}
 \makebox[0.15\textwidth]{\small 19.53}
 \makebox[0.15\textwidth]{\small 19.75}
  \\
  \vspace{1em}
 \includegraphics[width=0.15\textwidth]{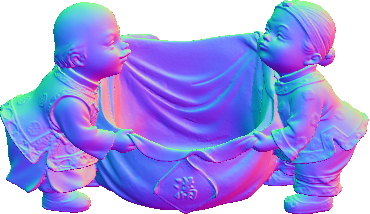}
 \includegraphics[width=0.15\textwidth]{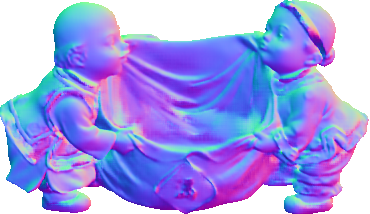}
 \includegraphics[width=0.15\textwidth]{images/Results/DiLiGenT/End_to_end/harvestPNGDiLiGenT_normal}
 \includegraphics[width=0.15\textwidth]{images/Results/DiLiGenT/UPS-FCN_ECCV/harvestPNGDiLiGenT_normal}
 \includegraphics[width=0.15\textwidth]{images/Results/DiLiGenT/compare/harvestPNGCVPR12Favaro_normal}
 \includegraphics[width=0.15\textwidth]{images/Results/DiLiGenT/compare/harvestPNGCVPR13Wu_normal}
  \\
  \includegraphics[width=0.15\textwidth]{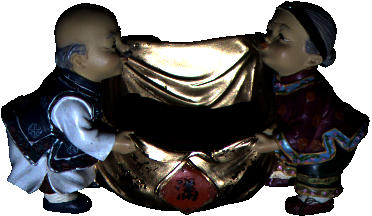}
 \includegraphics[width=0.15\textwidth]{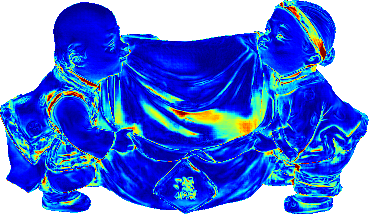}
 \includegraphics[width=0.15\textwidth]{images/Results/DiLiGenT/End_to_end/harvestPNGDiLiGenT_diff}
 \includegraphics[width=0.15\textwidth]{images/Results/DiLiGenT/UPS-FCN_ECCV/harvestPNGDiLiGenT_diff}
 \includegraphics[width=0.15\textwidth]{images/Results/DiLiGenT/compare/harvestPNGCVPR12Favaro_diff}
 \includegraphics[width=0.15\textwidth]{images/Results/DiLiGenT/compare/harvestPNGCVPR13Wu_diff}\\
 \makebox[0.15\textwidth]{\small (d) {\sc harvest}} 
 \makebox[0.15\textwidth]{\small 17.43}
 \makebox[0.15\textwidth]{\small 27.22}
 \makebox[0.15\textwidth]{\small 27.79}
 \makebox[0.15\textwidth]{\small 29.21}
 \makebox[0.15\textwidth]{\small 55.51}
\end{minipage}
    \begin{minipage}{0.02\textwidth} \centering
         \makebox[0.16\textwidth]{\small $0\degree$}\\ \vspace{0.2em}
         \includegraphics[width=\linewidth]{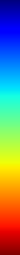} \\ \vspace{-0.4em}
         \makebox[0.16\textwidth]{\small$90\degree$}\\
    \end{minipage}
    \\
