# Supplementary material for: Self-calibrating Deep Photometric Stereo Networks
Source: arXiv:1903.07366 source file (2019-03-18)
Supplement: Supplementary file 5 [file res_qual_gourd.tex]

\makebox[0.19\textwidth]{\small Objects} 
    \makebox[0.19\textwidth]{\small UPS-FCN \cite{chen2018ps}}
    \makebox[0.19\textwidth]{\small UPS-FCN$_\text{deep+mask}$} 
    \makebox[0.19\textwidth]{\small SDPS-Net} 
    \makebox[0.15\textwidth]{\small SDPS-Net Dir. Err.} 
    \\
    \includegraphics[width=0.19\textwidth]{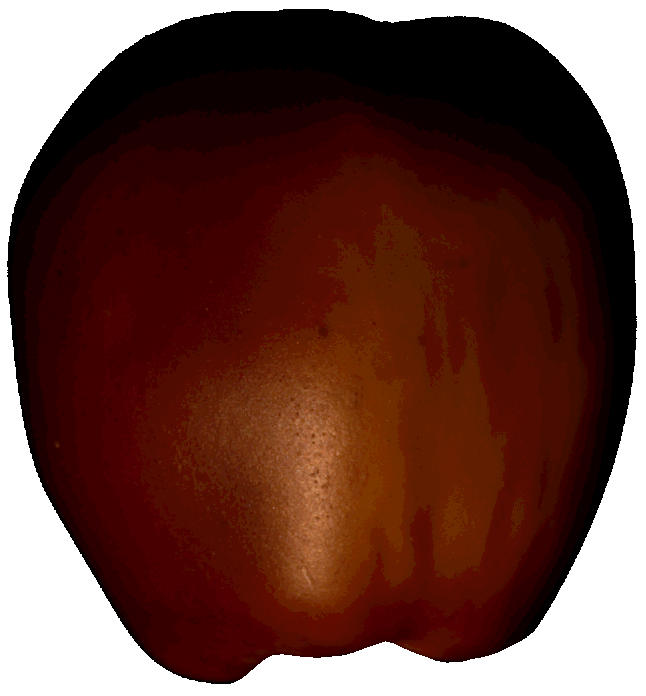}
    \includegraphics[width=0.19\textwidth]{images/Results/Gourd/UPS-FCN_ECCV/apple_Normal_DiLiGenT}
    \includegraphics[width=0.19\textwidth]{images/Results/Gourd/End_to_end/apple_Normal_DiLiGenT}
    \includegraphics[width=0.19\textwidth]{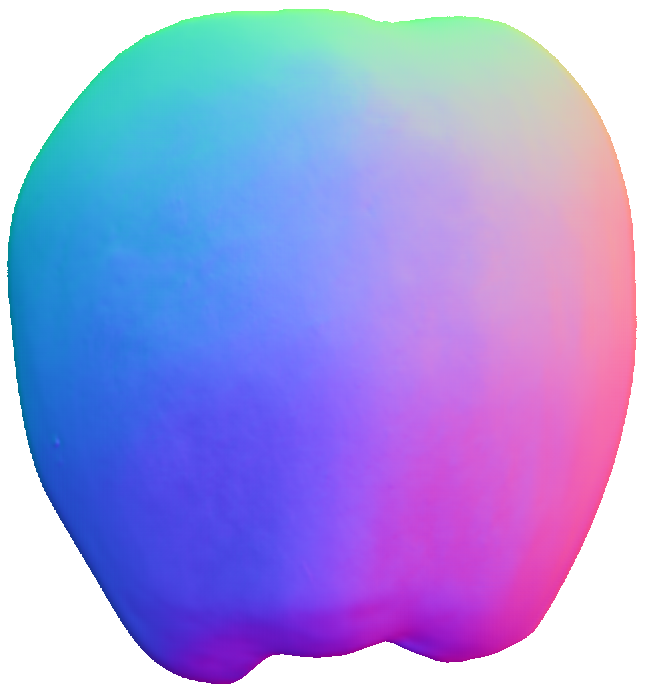}
    \includegraphics[width=0.13\textwidth]{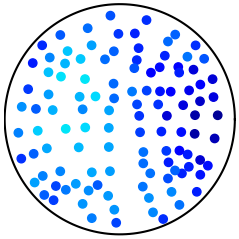}
    \begin{minipage}{0.012\textwidth} \centering
         \vspace{-6em} \makebox[0.16\textwidth]{\tiny $0\degree$}\\ \vspace{0.2em}
         \includegraphics[width=0.6\linewidth]{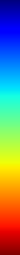} \\ \vspace{-0.4em}
         \makebox[0.16\textwidth]{\tiny$45\degree$}\\
    \end{minipage}
    \\ \vspace{-0.24em}\makebox[\textwidth]{\small (a) Apple} 
    \\
    \includegraphics[width=0.19\textwidth]{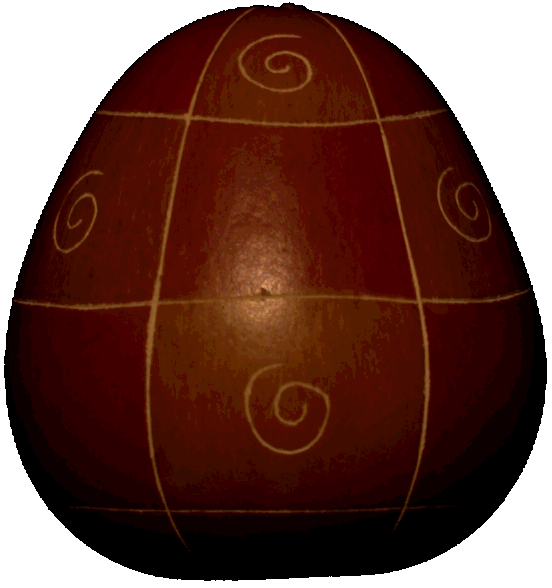}
    \includegraphics[width=0.19\textwidth]{images/Results/Gourd/UPS-FCN_ECCV/gourd1_Normal_DiLiGenT}
    \includegraphics[width=0.19\textwidth]{images/Results/Gourd/End_to_end/gourd1_Normal_DiLiGenT}
    \includegraphics[width=0.19\textwidth]{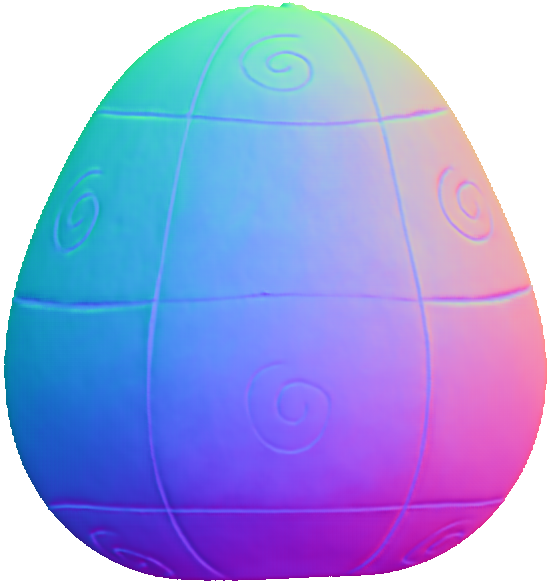}
    \includegraphics[width=0.13\textwidth]{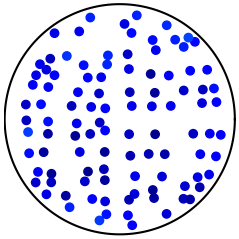}
    \begin{minipage}{0.012\textwidth} \centering
         \vspace{-6em} \makebox[0.16\textwidth]{\tiny $0\degree$}\\ \vspace{0.2em}
         \includegraphics[width=0.6\linewidth]{images/Results/color_bar} \\ \vspace{-0.4em}
         \makebox[0.16\textwidth]{\tiny$45\degree$}\\
    \end{minipage}
    \\ \vspace{-0.24em}\makebox[\textwidth]{\small (b) Gourd 1} 
    \\
    \includegraphics[width=0.19\textwidth]{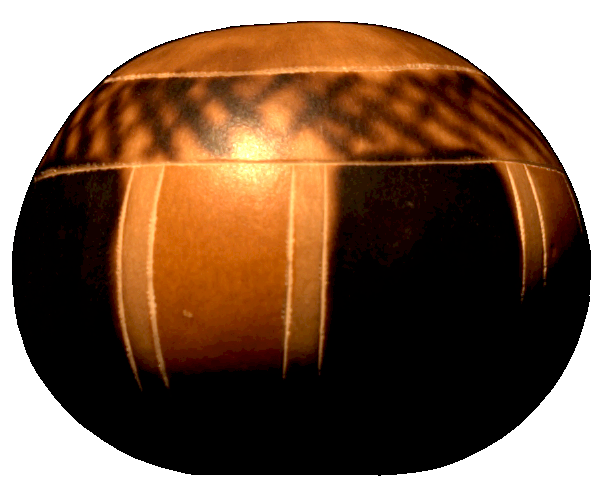}
    \includegraphics[width=0.19\textwidth]{images/Results/Gourd/UPS-FCN_ECCV/gourd2_Normal_DiLiGenT}
    \includegraphics[width=0.19\textwidth]{images/Results/Gourd/End_to_end/gourd2_Normal_DiLiGenT}
    \includegraphics[width=0.19\textwidth]{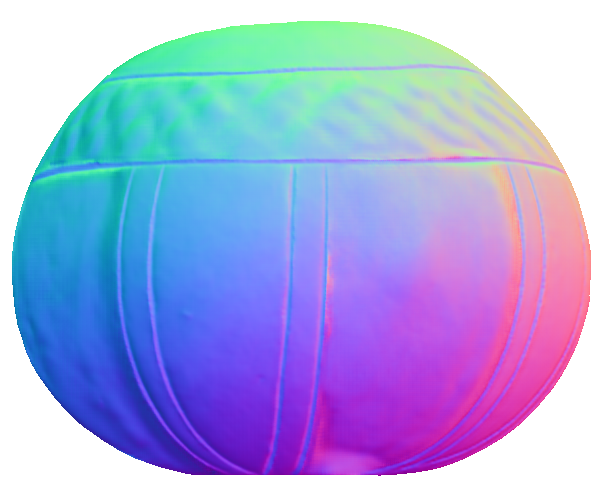}
    \includegraphics[width=0.13\textwidth]{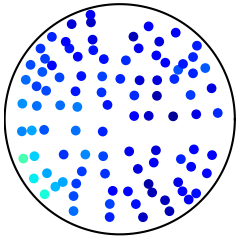}
    \begin{minipage}{0.012\textwidth} \centering
         \vspace{-6em} \makebox[0.16\textwidth]{\tiny $0\degree$}\\ \vspace{0.2em}
         \includegraphics[width=0.6\linewidth]{images/Results/color_bar} \\ \vspace{-0.4em}
         \makebox[0.16\textwidth]{\tiny$45\degree$}\\
    \end{minipage}
    \\ \vspace{-0.24em}\makebox[\textwidth]{\small (c) Gourd 2}
