# Supplementary material for: Self-calibrating Deep Photometric Stereo Networks
Source: arXiv:1903.07366 source file (2019-03-18)
Supplement: Supplementary file 6 [file qual_stage1.tex]

\makebox[0.21\textwidth]{\small Objects} 
    \makebox[0.21\textwidth]{\small UPS-FCN \cite{chen2018ps}}
    \makebox[0.21\textwidth]{\small UPS-FCN$_\text{deep+mask}$} 
    \makebox[0.21\textwidth]{\small SDPS-Net} 
    \makebox[0.10\textwidth]{\small SDPS-Net Dir. Err.} 
    \\
    \includegraphics[width=0.21\textwidth]{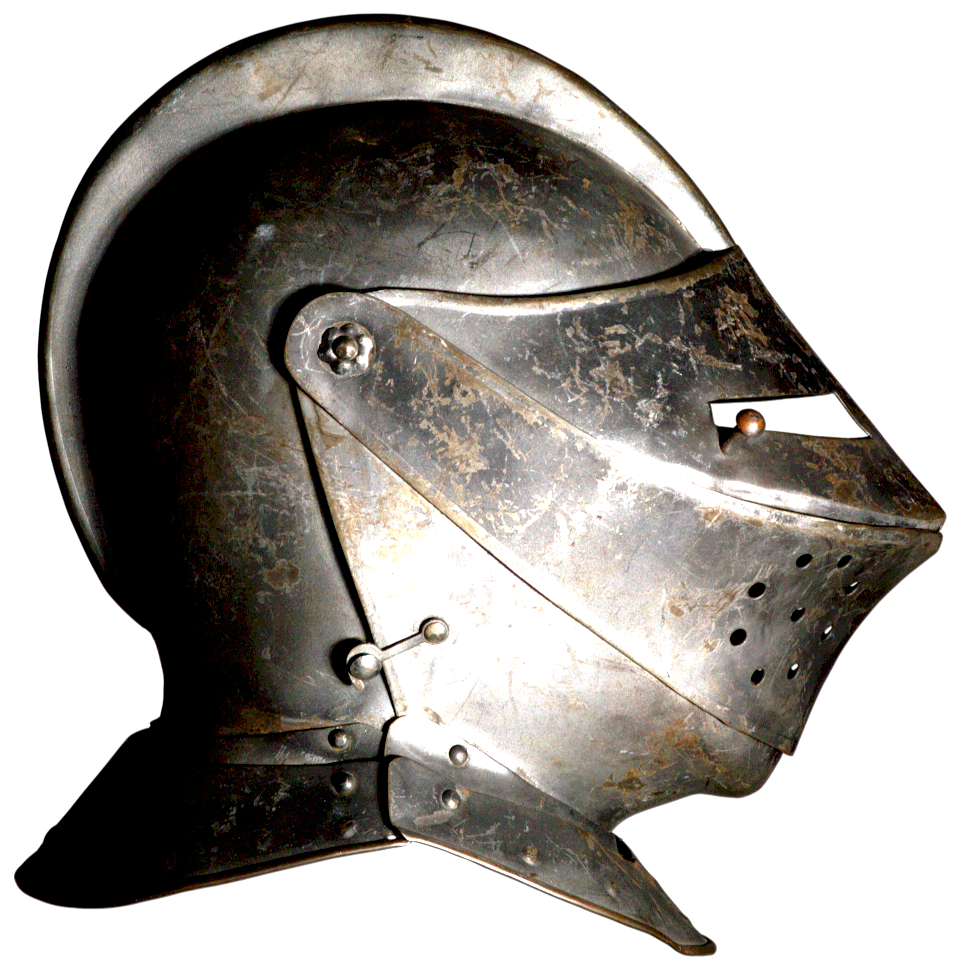}
    \includegraphics[width=0.21\textwidth]{images/Results/LightStage/UPS-FCN_ECCV/helmet_side_left_Normal_DiLiGenT}
    \includegraphics[width=0.21\textwidth]{images/Results/LightStage/End_to_end/helmet_side_left_Normal_DiLiGenT}
    \includegraphics[width=0.21\textwidth]{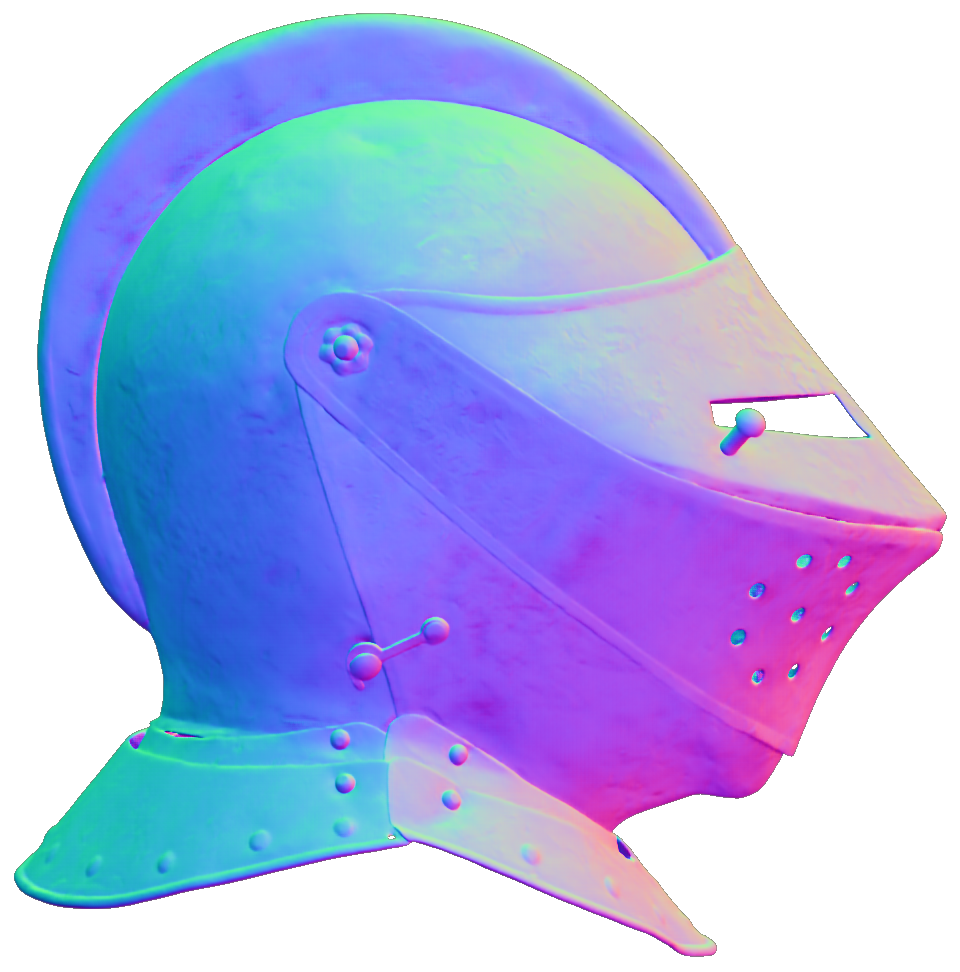}
    \raisebox{0.2\height}{\includegraphics[width=0.10\textwidth]{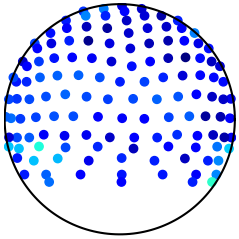}}
    \begin{minipage}{0.012\textwidth} \centering
         \vspace{-6em} \makebox[0.16\textwidth]{\tiny $0\degree$}\\ \vspace{0.2em}
         \includegraphics[width=0.6\linewidth]{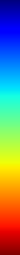} \\ \vspace{-0.4em}
         \makebox[0.16\textwidth]{\tiny$45\degree$}\\
    \end{minipage}
    \\ \makebox{\small (a) {\sc Helmet Side}} \\
    \includegraphics[width=0.21\textwidth]{images/Results/LightStage/{4.0_helmet_front_left_helmet_front_left_0082}.png}
    \includegraphics[width=0.21\textwidth]{images/Results/LightStage/UPS-FCN_ECCV/helmet_front_left_Normal_DiLiGenT}
    \includegraphics[width=0.21\textwidth]{images/Results/LightStage/End_to_end/helmet_front_left_Normal_DiLiGenT}
    \includegraphics[width=0.21\textwidth]{images/Results/LightStage/SCPS/helmet_front_left_Normal_DiLiGenT}
    \raisebox{0.6\height}{\includegraphics[width=0.10\textwidth]{images/Results/LightStage/SCPS/helmet_front_left}}
    \begin{minipage}{0.012\textwidth} \centering
         \vspace{-10em} \makebox[0.16\textwidth]{\tiny $0\degree$}\\ \vspace{0.2em}
         \includegraphics[width=0.6\linewidth]{images/Results/color_bar} \\ \vspace{-0.4em}
         \makebox[0.16\textwidth]{\tiny$45\degree$}\\
    \end{minipage}
    \\ \makebox{\small (b) {\sc Helmet Front}} \\
    \includegraphics[width=0.21\textwidth]{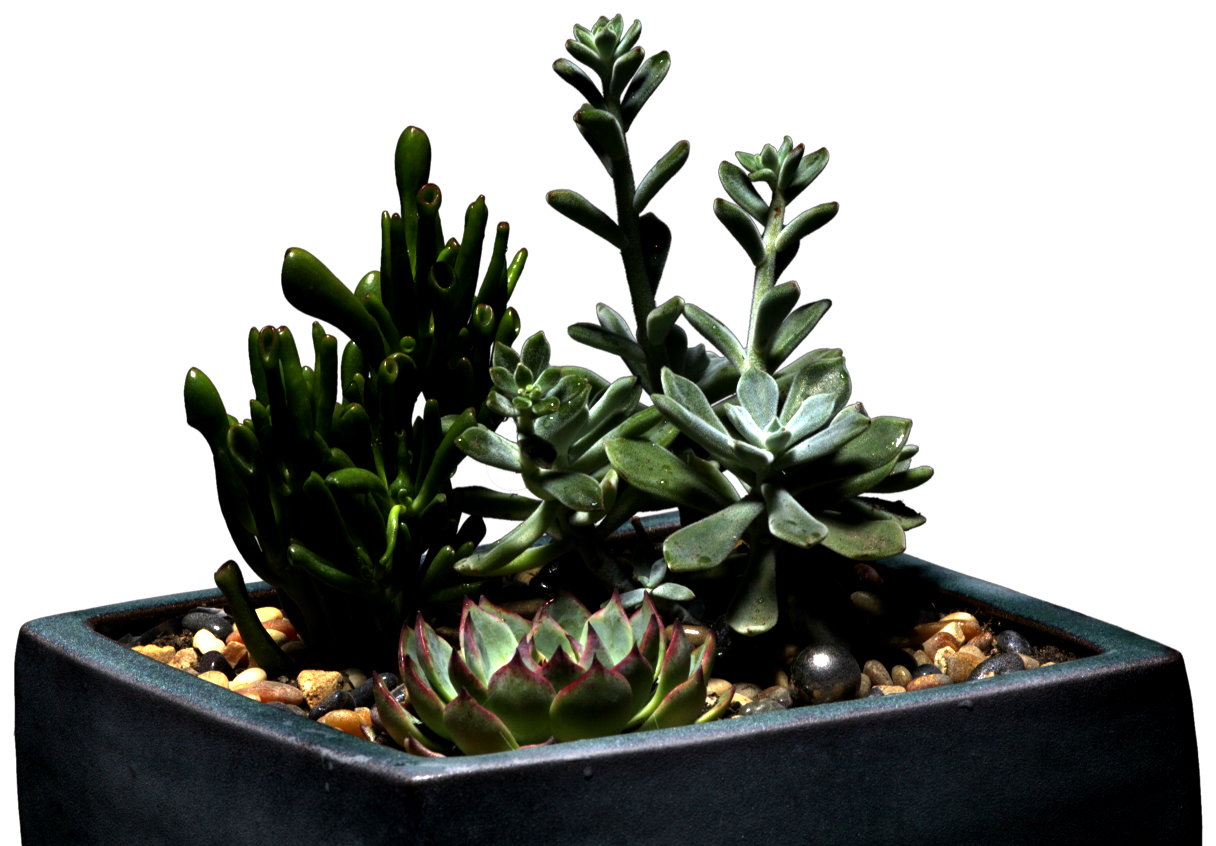}
    \includegraphics[width=0.21\textwidth]{images/Results/LightStage/UPS-FCN_ECCV/plant_left_Normal_DiLiGenT}
    \includegraphics[width=0.21\textwidth]{images/Results/LightStage/End_to_end/plant_left_Normal_DiLiGenT}
    \includegraphics[width=0.21\textwidth]{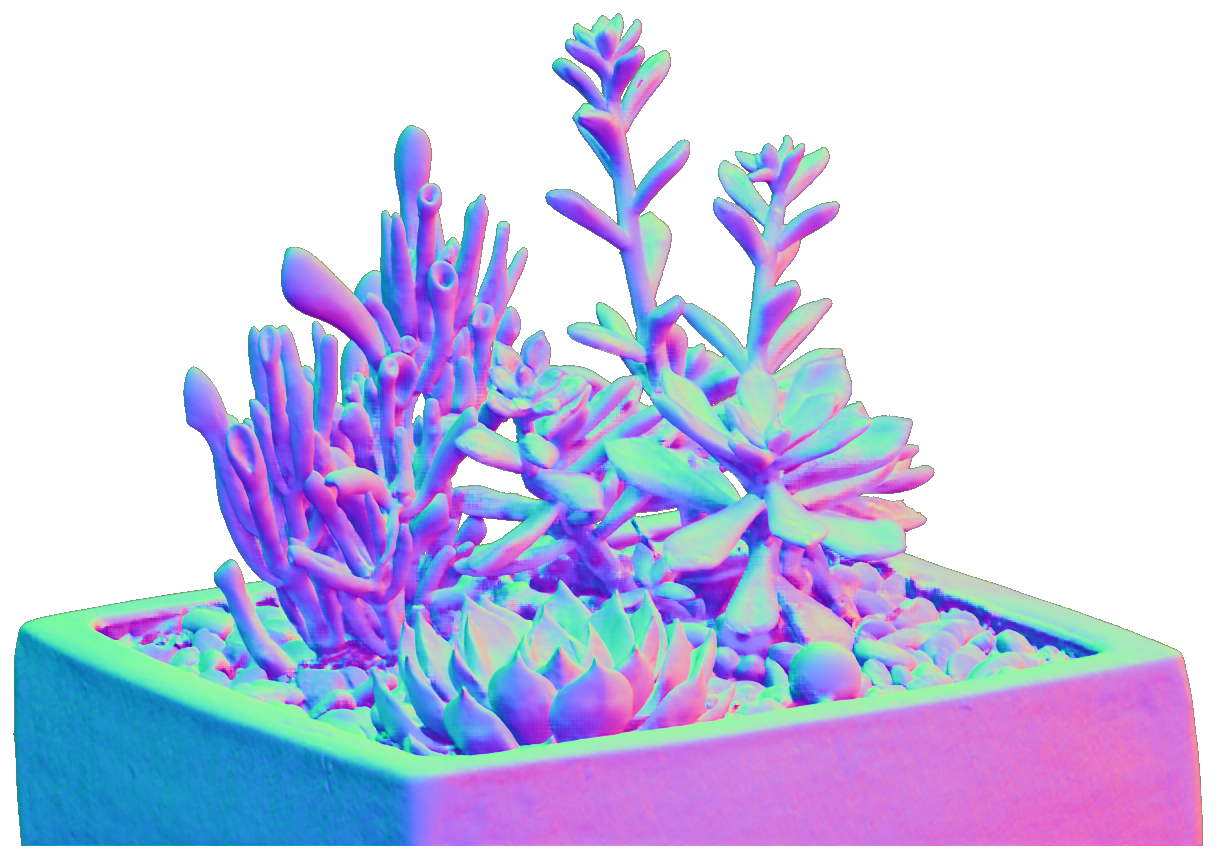}
    \raisebox{0.0\height}{\includegraphics[width=0.10\textwidth]{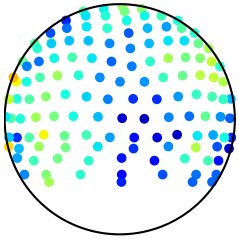}}
    \begin{minipage}{0.012\textwidth} \centering
         \vspace{-6em} \makebox[0.16\textwidth]{\tiny $0\degree$}\\ \vspace{0.2em}
         \includegraphics[width=0.6\linewidth]{images/Results/color_bar} \\ \vspace{-0.4em}
         \makebox[0.16\textwidth]{\tiny$45\degree$}\\
    \end{minipage}
    \\ \makebox{\small (c) {\sc Plant}} \\
